# Supplementary material for: Measuring Psychological Depth in Language Models
Source: arXiv:2406.12680 source file (2024-10-04)
Supplement: Supplementary file 1 [file framework_v1_sm.tex]

% sreya's version
\section{Related Work}

Rubrics serve as a key instrument for evaluating writing, so we chose to create a set of metrics that encompass notable attributes pertinent to our study of evaluating LLMs at a psychological depth level. To come up with a list of metrics we consulted several psychology papers to get attributes that have an impact on defining what the term ‘psychological depth’ meant. After filtering and consolidating, we finalized 5 different metrics to use in our study: authenticity, empathy, engagement, emotion provoking, and narrative complexity. 

\textbf{Authenticity:} This metric focuses on asking if the writing felt true to real human experiences, regardless of whether the reader personally experienced the situation. To be authentic also targets the idea of representing a psychological process that’s believable. A study reported that narratives written authentically and inauthentically coincided with their reported self-scores\cite{Wilt2019}. This suggests that humans can clearly distinguish between authentic and inauthentic writing, which shows how important authenticity can be to an audience. 

\textbf{Empathy:} It measures how well the audience was able to empathize with the characters and their situations in the text. This also tests the possibility of the reader being able to lead to new introspection or new insights about the world. A study states how empathetic people mention a lot of negative feelings, such as feeling overwhelmed or isolation \cite{Yaden2023}. This proves that writing infused with empathy can help bond readers and writers over painful experiences which unlocks the writing piece’s ability to get readers to understand their point of view. 

\textbf{Engagement:} Choosing this measurement was important to see how well the writing piece was able to keep the reader’s focus at an emotional and psychological level. In a study, researchers were able to find a positive correlation between engaging stories and higher engagement scores, which also confirms engagement as a significant factor to use.\cite{Sukalla2015}.  

\textbf{Emotion provoking:} This measurement forces the readers in the study to distinguish between describing the nuances of a character’s state rather than using simple terms that give surface-level writing. The significance of the metric on one’s psychological state can be seen in a study such that shows that writing about emotional experiences show significant improvement on mental and physical health\cite{Pennebaker1997}. This proves that using emotion-provoking is a key component in evaluating psychological depth as it directly correlates to mental health. 

\textbf{Narrative complexity:} Using narrative complexity as a metric in this study puts a lens on characters having multifaceted personalities and exhibiting internal conflicts. Stories should also aim to explore more complicated relationships between characters rather than stereotypical ones. A study points out how films evoke dissonant cognitions in their audience\cite{Kiss2017}. This is a clear indicator of the possible mental effects the style of a narrative can have.
